# Supplementary material for: Search for transient ultralight dark matter signatures with networks of precision measurement devices using a Bayesian statistics method
Source: arXiv:1803.10264 ancillary file (2018-03-27)
Supplement: Supplementary file 1 [file BayesianSupplement.pdf]

# GPS satellite clock noise characteristics

## Supplement to: *Search for transient ultralight dark matter signatures with networks of precision measurement devices using a Bayesian statistics method*

B. M. Roberts, G. Blewitt, C. Dailey, & A. Derevianko

Department of Physics, University of Nevada, Reno, 89557, USA

March 26, 2018

Noise characteristics (standard deviations, autocorrelation, Allan variance, histograms, power spectrums) for the GPS satellite clocks. Broken up by SVN, clock, block, and reference clock. Except where stated, the analysis includes data from the period 18 July 2004 – 29 July 2017. In total, this spans 6,295 days, and includes 186,024 clock-days of data (or, about half a billion clock-epochs). Not all days were actually included in the calculations. Excluded are clocks that had 10 or more missing data points in the given day, or any outliers larger than 100 ns. The effect of these exclusions is rather minor, see section 1.1.

We use data made publicly available by JPL [1]. JPL provides a file [2] that links each GPS "slot" with the particular satellite (by space-vehicle number, SVN) that occupies the slot on a given day, and which clock (Rb or Cs) was employed. However, the clock assignments are not always accurate. The correct clock assignments are given by the US Navigation Center's operational advisories [3]. We provide a simple python script that automatically reconciles the two sources to give accurate SVN and clock assignments for each GPS satellite [4].

## Contents

1 Standard deviations 1

1.1 Exclusions and change over time . . . . . 5

2 Auto correlation functions 6

3 Allan variance 10

4 Histogram 13

5 Power spectrums 16

6 Cross-clock correlations 19

# 1 Standard deviations

Presented are the standard deviations for the first- and second-order differenced clock data. Also shown are the $1\sigma$ uncertainties in these values (daily variation). The standard deviations are also presented for each SVN separately for the USN3 reference clock (the most common reference used).

The column "days" is the total number of days of data included for the given clock. The "excluded" column is the numbers of days that were excluded (either because of huge outliers, or because they were missing data points/incomplete days).

For the Rb clocks, the $\sigma$ for the second-order differenced data is larger than for the first-order differenced data, roughly by a factor of $\sqrt{2}$, just as we would expect, since to a reasonable approximation, the Rb data is stationary after first-order differencing. For the Cs block II and IIA clocks, however, the standard deviation becomes smaller

for the second-order differenced data, which is also what we expect, since the Cs data is not sufficiently stationary after first-order differencing.

Table 1: Summary standard deviations for the first- and second-order differenced clock data for the RbII satellites, by block, reference clock (not all reference clocks shown here), and SVN. "av" in the SVN column means averaged over all SVNs, and "Hmas" in the ref. column means averaged over all (H-maser) reference clocks. Values given are the averages over all available clock-days for the given block/reference combination; numbers in parenthesis are the ($1\sigma$) daily-variation uncertainties in these values [e.g., $0.0261(25) = 0.0261 \pm 0.0025$] .

| Block | SVN | Ref. | Days | Excluded | $\sigma^{(1)}$/ns | $\sigma^{(2)}$/ns |
|---|---|---|---|---|---|---|
| RbII | 15 | USN3 | 20 | 95 | 0.0266(28) | 0.0374(42) |
| RbII | 17 | USN3 | 146 | 59 | 0.0512(193) | 0.0743(285) |
| RbII | av | USN3 | 166 | 154 | 0.0482(198) | 0.0698(293) |
| RbII | av | Hmas | 179 | 159 | 0.0477(195) | 0.0691(289) |

Table 2: Summary standard deviations for the first- and second-order differenced clock data for the RbIIA satellites.

| Block | SVN | Ref. | Days | Excluded | $\sigma^{(1)}$/ns | $\sigma^{(2)}$/ns |
|---|---|---|---|---|---|---|
| RbIIA | 23 | USN3 | 1902 | 661 | 0.0283(48) | 0.0432(90) |
| RbIIA | 25 | USN3 | 969 | 361 | 0.0372(109) | 0.0550(157) |
| RbIIA | 26 | USN3 | 2709 | 868 | 0.0380(102) | 0.0559(152) |
| RbIIA | 27 | USN3 | 306 | 94 | 0.0522(269) | 0.0697(272) |
| RbIIA | 29 | USN3 | 649 | 208 | 0.0429(80) | 0.0645(127) |
| RbIIA | 30 | USN3 | 503 | 135 | 0.0402(111) | 0.0603(160) |
| RbIIA | 31 | USN3 | 193 | 74 | 0.0306(123) | 0.0441(125) |
| RbIIA | 33 | USN3 | 117 | 48 | 0.0388(67) | 0.0561(64) |
| RbIIA | 34 | USN3 | 2955 | 624 | 0.0473(27) | 0.0687(53) |
| RbIIA | 35 | USN3 | 1364 | 469 | 0.0289(78) | 0.0438(138) |
| RbIIA | 36 | USN3 | 2736 | 606 | 0.0488(98) | 0.0712(138) |
| RbIIA | 37 | USN3 | 950 | 215 | 0.0349(54) | 0.0530(103) |
| RbIIA | 40 | USN3 | 135 | 38 | 0.0547(16) | 0.0786(28) |
| RbIIA | av | AMC2 | 1163 | 334 | 0.0362(117) | 0.0525(163) |
| RbIIA | av | KOKB | 33 | 12 | 0.0441(72) | 0.0668(113) |
| RbIIA | av | PTBB | 37 | 7 | 0.0443(88) | 0.0618(147) |
| RbIIA | av | TWTF | 47 | 15 | 0.0417(167) | 0.0604(182) |
| RbIIA | av | USN3 | 15489 | 4434 | 0.0400(117) | 0.0590(164) |
| RbIIA | av | USN7 | 49 | 18 | 0.0307(87) | 0.0452(118) |
| RbIIA | av | USNO | 56 | 15 | 0.0381(113) | 0.0564(170) |
| RbIIA | av | WTZR | 35 | 10 | 0.0428(134) | 0.0640(208) |
| RbIIA | av | Hmas | 16909 | 4845 | 0.0398(118) | 0.0586(165) |

Table 3: Summary standard deviations for the first- and second-order differenced clock data for the RbIIR satellites.

| Block | SVN | Ref. | Days | Excluded | $\sigma^{(1)}$/ns | $\sigma^{(2)}$/ns |
|---|---|---|---|---|---|---|
| RbIIR | 41 | USN3 | 3529 | 67 | 0.0669(45) | 0.0892(73) |
| RbIIR | 43 | USN3 | 3486 | 106 | 0.0762(103) | 0.1042(165) |
| RbIIR | 44 | USN3 | 3527 | 74 | 0.0690(53) | 0.0909(81) |
| RbIIR | 45 | USN3 | 3359 | 229 | 0.0927(74) | 0.1198(105) |
| RbIIR | 46 | USN3 | 3506 | 91 | 0.0701(36) | 0.0919(44) |
| RbIIR | 47 | USN3 | 3521 | 80 | 0.0767(116) | 0.0987(131) |
| RbIIR | 48 | USN3 | 2302 | 31 | 0.0709(27) | 0.0951(42) |
| RbIIR | 50 | USN3 | 1647 | 193 | 0.0792(80) | 0.1082(124) |
| RbIIR | 51 | USN3 | 3535 | 59 | 0.0711(62) | 0.0927(87) |
| RbIIR | 52 | USN3 | 2808 | 15 | 0.0673(31) | 0.0905(47) |
| RbIIR | 53 | USN3 | 3085 | 81 | 0.0738(60) | 0.0982(80) |
| RbIIR | 54 | USN3 | 3501 | 94 | 0.0817(94) | 0.1060(113) |
| RbIIR | 55 | USN3 | 2443 | 24 | 0.0734(25) | 0.0982(36) |
| RbIIR | 56 | USN3 | 3515 | 75 | 0.0761(109) | 0.1047(164) |
| RbIIR | 57 | USN3 | 2390 | 12 | 0.0724(57) | 0.0974(85) |
| RbIIR | 58 | USN3 | 2706 | 62 | 0.0826(83) | 0.1137(127) |
| RbIIR | 59 | USN3 | 3541 | 51 | 0.0692(53) | 0.0917(84) |
| RbIIR | 60 | USN3 | 3542 | 49 | 0.0659(72) | 0.0890(122) |
| RbIIR | 61 | USN3 | 3410 | 51 | 0.0657(37) | 0.0882(55) |
| RbIIR | av | AMC2 | 8265 | 1796 | 0.0752(82) | 0.1008(119) |
| RbIIR | av | KOKB | 99 | 0 | 0.0706(130) | 0.0936(200) |
| RbIIR | av | NIST | 47 | 65 | 0.0722(56) | 0.0970(75) |
| RbIIR | av | PTBB | 117 | 7 | 0.0731(124) | 0.0953(189) |
| RbIIR | av | TWTF | 155 | 1 | 0.0695(91) | 0.0915(122) |
| RbIIR | av | USN3 | 59353 | 1448 | 0.0736(98) | 0.0979(134) |
| RbIIR | av | USN7 | 6690 | 3488 | 0.0754(71) | 0.1014(100) |
| RbIIR | av | USNO | 178 | 3 | 0.0735(97) | 0.0977(127) |
| RbIIR | av | WTZR | 303 | 57 | 0.0767(80) | 0.1033(118) |
| RbIIR | av | Hmas | 75207 | 6865 | 0.0739(95) | 0.0986(131) |

Table 4: Summary standard deviations for the first- and second-order differenced clock data for the RbIIF satellites.

| Block | SVN | Ref. | Days | Excluded | $\sigma^{(1)}$/ns | $\sigma^{(2)}$/ns |
|---|---|---|---|---|---|---|
| RbIIF | 62 | USN7 | 530 | 3 | 0.0152(21) | 0.0253(39) |
| RbIIF | 63 | USN7 | 527 | 9 | 0.0124(9) | 0.0197(13) |
| RbIIF | 64 | USN7 | 528 | 5 | 0.0129(6) | 0.0206(11) |
| RbIIF | 66 | USN7 | 522 | 10 | 0.0129(16) | 0.0209(29) |
| RbIIF | 67 | USN7 | 532 | 4 | 0.0151(19) | 0.0247(33) |
| RbIIF | 68 | USN7 | 528 | 8 | 0.0148(21) | 0.0241(38) |
| RbIIF | 69 | USN7 | 525 | 8 | 0.0120(8) | 0.0192(13) |
| RbIIF | 70 | USN7 | 444 | 1 | 0.0141(23) | 0.0230(42) |
| RbIIF | 71 | USN7 | 527 | 5 | 0.0173(13) | 0.0285(23) |
| RbIIF | 73 | USN7 | 524 | 3 | 0.0130(9) | 0.0203(13) |
| RbIIF | av | AMC2 | 3327 | 81 | 0.0117(15) | 0.0185(28) |
| RbIIF | av | NIST | 60 | 0 | 0.0157(24) | 0.0252(43) |
| RbIIF | av | USN3 | 3200 | 259 | 0.0132(28) | 0.0213(42) |
| RbIIF | av | USN7 | 5188 | 56 | 0.0140(24) | 0.0226(41) |
| RbIIF | av | WTZR | 120 | 1 | 0.0161(19) | 0.0264(35) |
| RbIIF | av | Hmas | 11909 | 397 | 0.0132(25) | 0.0212(42) |

Table 5: Summary standard deviations for the first- and second-order differenced clock data for the CsII satellites.

| Block | SVN | Ref. | Days | Excluded | $\sigma^{(1)}$/ns | $\sigma^{(2)}$/ns |
|---|---|---|---|---|---|---|
| CsII | 15 | USN3 | 505 | 222 | 0.0834(24) | 0.0715(48) |
| CsII | av | USN3 | 505 | 222 | 0.0834(24) | 0.0715(48) |
| CsII | av | AMC2 | 22 | 7 | 0.0825(20) | 0.0665(33) |
| CsII | av | Hmas | 538 | 231 | 0.0833(24) | 0.0712(48) |

Table 6: Summary standard deviations for the first- and second-order differenced clock data for the CsIIA satellites.

| Block | SVN | Ref. | Days | Excluded | $\sigma^{(1)}$/ns | $\sigma^{(2)}$/ns |
|---|---|---|---|---|---|---|
| CsIIA | 24 | USN3 | 1984 | 454 | 0.0811(29) | 0.0765(63) |
| CsIIA | 25 | USN3 | 415 | 106 | 0.0885(101) | 0.0899(68) |
| CsIIA | 27 | USN3 | 1783 | 672 | 0.0813(55) | 0.0719(162) |
| CsIIA | 29 | USN3 | 109 | 88 | 0.1113(24) | 0.1421(49) |
| CsIIA | 30 | USN3 | 1369 | 420 | 0.0958(93) | 0.0983(195) |
| CsIIA | 31 | USN3 | 47 | 40 | 0.1056(30) | 0.0702(13) |
| CsIIA | 32 | USN3 | 913 | 365 | 0.0773(53) | 0.0476(54) |
| CsIIA | 33 | USN3 | 2701 | 629 | 0.0967(128) | 0.1110(249) |
| CsIIA | 35 | USN3 | 302 | 88 | 0.0820(41) | 0.0744(65) |
| CsIIA | 38 | USN3 | 2500 | 1058 | 0.0962(83) | 0.1016(183) |
| CsIIA | 39 | USN3 | 2575 | 849 | 0.0878(126) | 0.0876(219) |
| CsIIA | 40 | USN3 | 2617 | 787 | 0.0863(113) | 0.0900(198) |
| CsIIA | av | AMC2 | 582 | 569 | 0.0886(128) | 0.0885(273) |
| CsIIA | av | KOKB | 40 | 12 | 0.0904(135) | 0.0933(295) |
| CsIIA | av | PTBB | 39 | 6 | 0.0868(103) | 0.0832(206) |
| CsIIA | av | TWTF | 53 | 16 | 0.0903(129) | 0.0929(256) |
| CsIIA | av | USN3 | 17315 | 5589 | 0.0889(119) | 0.0896(246) |
| CsIIA | av | USNO | 66 | 11 | 0.0909(121) | 0.0922(263) |
| CsIIA | av | WTZR | 20 | 17 | 0.0870(50) | 0.0870(107) |
| CsIIA | av | Hmas | 18121 | 6344 | 0.0889(119) | 0.0896(248) |

Table 7: Summary standard deviations for the first- and second-order differenced clock data for the CsIIF satellites.

| Block | SVN | Ref. | Days | Excluded | $\sigma^{(1)}$/ns | $\sigma^{(2)}$/ns |
|---|---|---|---|---|---|---|
| CsIIF | 65 | AMC2 | 128 | 317 | 0.1000(15) | 0.1387(25) |
| CsIIF | 72 | AMC2 | 163 | 9 | 0.0731(15) | 0.1012(20) |
| CsIIF | av | AMC2 | 291 | 335 | 0.0849(134) | 0.1177(188) |
| CsIIF | av | USN3 | 625 | 145 | 0.0983(18) | 0.1363(29) |
| CsIIF | av | USN7 | 540 | 522 | 0.0757(80) | 0.1051(113) |
| CsIIF | av | Hmas | 1477 | 1022 | 0.0872(128) | 0.1210(178) |

## 1.1 Exclusions and change over time

The effect of excluding data is shown in Table 8. For the "heavy" exclusions, days that had any missing data points, had standard deviations $\sigma > 0.2\,\mathrm{ns}$, or had any outliers with $d^{(1)} > 25\,\mathrm{ns}$ were excluded. While this does affect the stability in the standard deviations (i.e., the uncertainty in the standard deviation), it has only negligible impact on the values.

How the clock performance changes over time is detailed in Tables 9 and 10 for the Rb and Cs clocks, averaged over all SVNs. The same is shown for a single SVN of a Rb-IIR clock (SVN:51) in Table 11; these satellites (which are the worst in this regard) seem to degrade substantially over the years.

Table 8: Summary of how the standard deviations (first-order differenced data) change depending on how we exclude days. The first column includes all days, and the second excludes about 30% of the days.

| Block | No Excl. | "Heavy" Excl. |
|---|---|---|
| RbII | 0.0429(179) | 0.0477(195) |
| RbIIA | 0.0398(132) | 0.0398(118) |
| RbIIR | 0.0750(106) | 0.0739(95) |
| RbIIF | 0.0135(45) | 0.0132(25) |
| CsII | 0.0831(42) | 0.0833(24) |
| CsIIA | 0.0889(138) | 0.0889(119) |
| CsIIF | 0.0938(212) | 0.0872(128) |

Table 9: Variations of the Rb standard deviations over time. Averaged over all SVNs.

| Year/month | RbIIF | RbIIR | RbIIA | RbII |
|---|---|---|---|---|
| 2000/05–2004/07 | | 0.0609(174) | 0.0452(244) | 0.0440(188) |
| 2004/07–2008/10 | | 0.0714(111) | 0.0410(113) | 0.0477(195) |
| 2008/10–2012/12 | 0.0139(41) | 0.0737(85) | 0.0390(114) | |
| 2012/12–2017/07 | 0.0131(22) | 0.0762(84) | 0.0375(134) | |

Table 10: Variations of the Cs standard deviations over time. Averaged over all SVNs.

| Year/month | CsIIF | CsIIA | CsII |
|---|---|---|---|
| 2000/05–2004/07 | | 0.0851(165) | 0.0957(257) |
| 2004/07–2008/10 | | 0.0887(138) | 0.0833(24) |
| 2008/10–2012/12 | 0.0956(11) | 0.0901(100) | |
| 2012/12–2017/07 | 0.0870(129) | 0.0853(50) | |

Table 11: Variations of the standard deviations for one particular Rb-IIR SVN (51) over time. RbIIR is the "worst offender" in this regard, and changes quite substantially over time.

| RbIIR : 51 | USN3 | AMC2 |
|---|---|---|
| 2000/05–2004/07 | 0.0498(6) | 0.0472(12) |
| 2004/07–2008/10 | 0.0667(75) | 0.0658(85) |
| 2008/10–2012/12 | 0.0735(23) | 0.0725(21) |
| 2012/12–2017/07 | 0.0753(20) | 0.0755(22) |

## 2 Auto correlation functions

First- and second-order differenced data:

$$d_j^{(1)} \equiv d_j^{(0)} - d_{j-1}^{(0)}, \tag{1}$$

$$d_j^{(2)} \equiv d_{j+1}^{(0)} - 2d_j^{(0)} + d_{j-1}^{(0)}, \tag{2}$$

where $d_j^{(0)}$ is the original clock bias time-series.

Auto-correlation function (ACF):

$$A^i(\Delta t) = \sum_{j=0}^{J-\tau-1} \frac{\left(d_j^i - \bar{d}^i\right)\left(d_{j+\tau}^i - \bar{d}^i\right)}{\sigma_i^2 (J-\tau)}, \tag{3}$$

where $\bar{d}_i$ is the average value of the time-series data $\{d_{ij}\}$, $\Delta t = \tau\tau_0$ ($\tau \in \mathbb{I}$, and for our current 30 s sampled data, $\tau_0 = 30\,\mathrm{s}$), and $J$ is the total number of data points for each clock per day. For the 30 s data, $J = 2880$. (Here, $\sigma_i$ is the standard deviation of the clock data, not the formal error.) Rb: Figs. 1–3; Cs: Figs. 4–5.

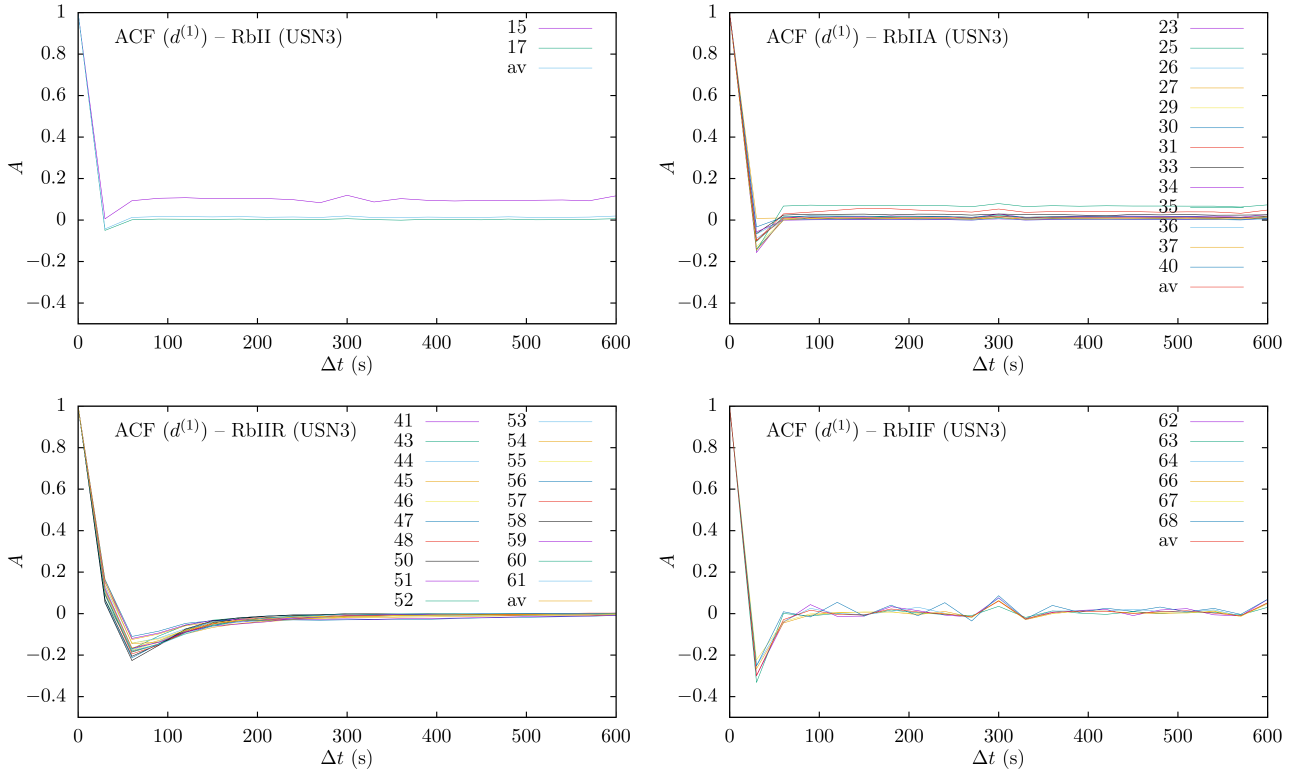


Figure 1: Rb autocorrelation functions, using first-order differenced data. Each plot is for a particular Rb satellite block; each SVN is shown separately. Line labeled "av" is the average over all SNVs.

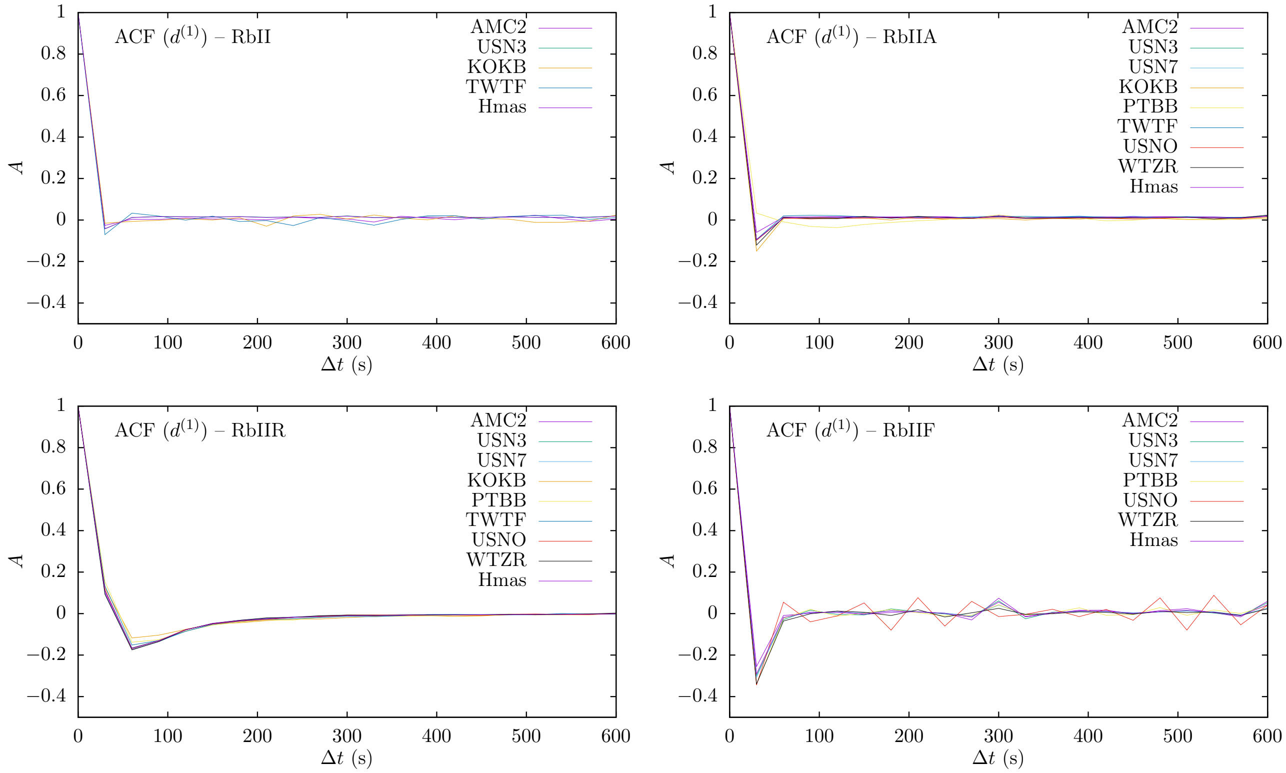


Figure 2: Rb autocorrelation functions, using first-order differenced data. Each plot is for a particular Rb satellite block; each reference clock is shown separately. Line labeled "Hmas" is the average over all (H-maser) reference clocks.

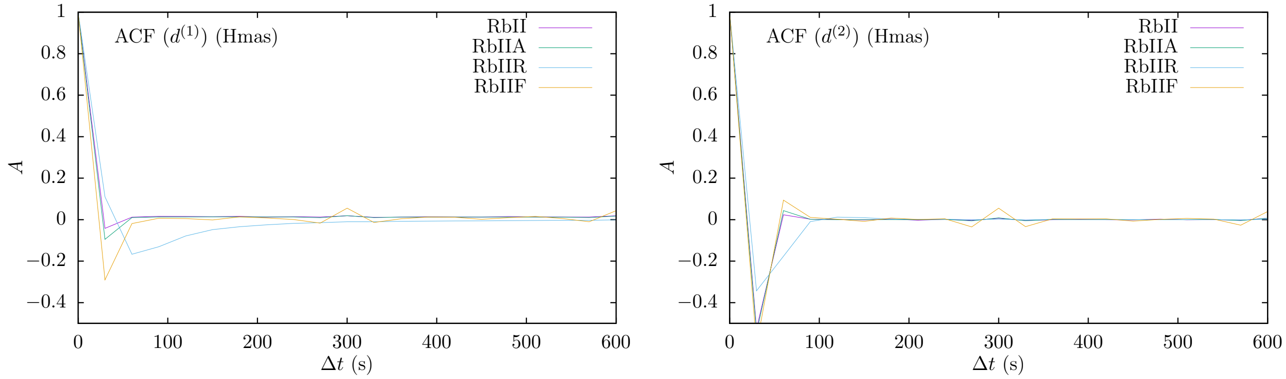


Figure 3: Rb autocorrelation functions for each Rb satellite block, averaged over all SVN's and all (H-maser) reference clocks. Left: using first-order differencing. Right: using second-order differencing.

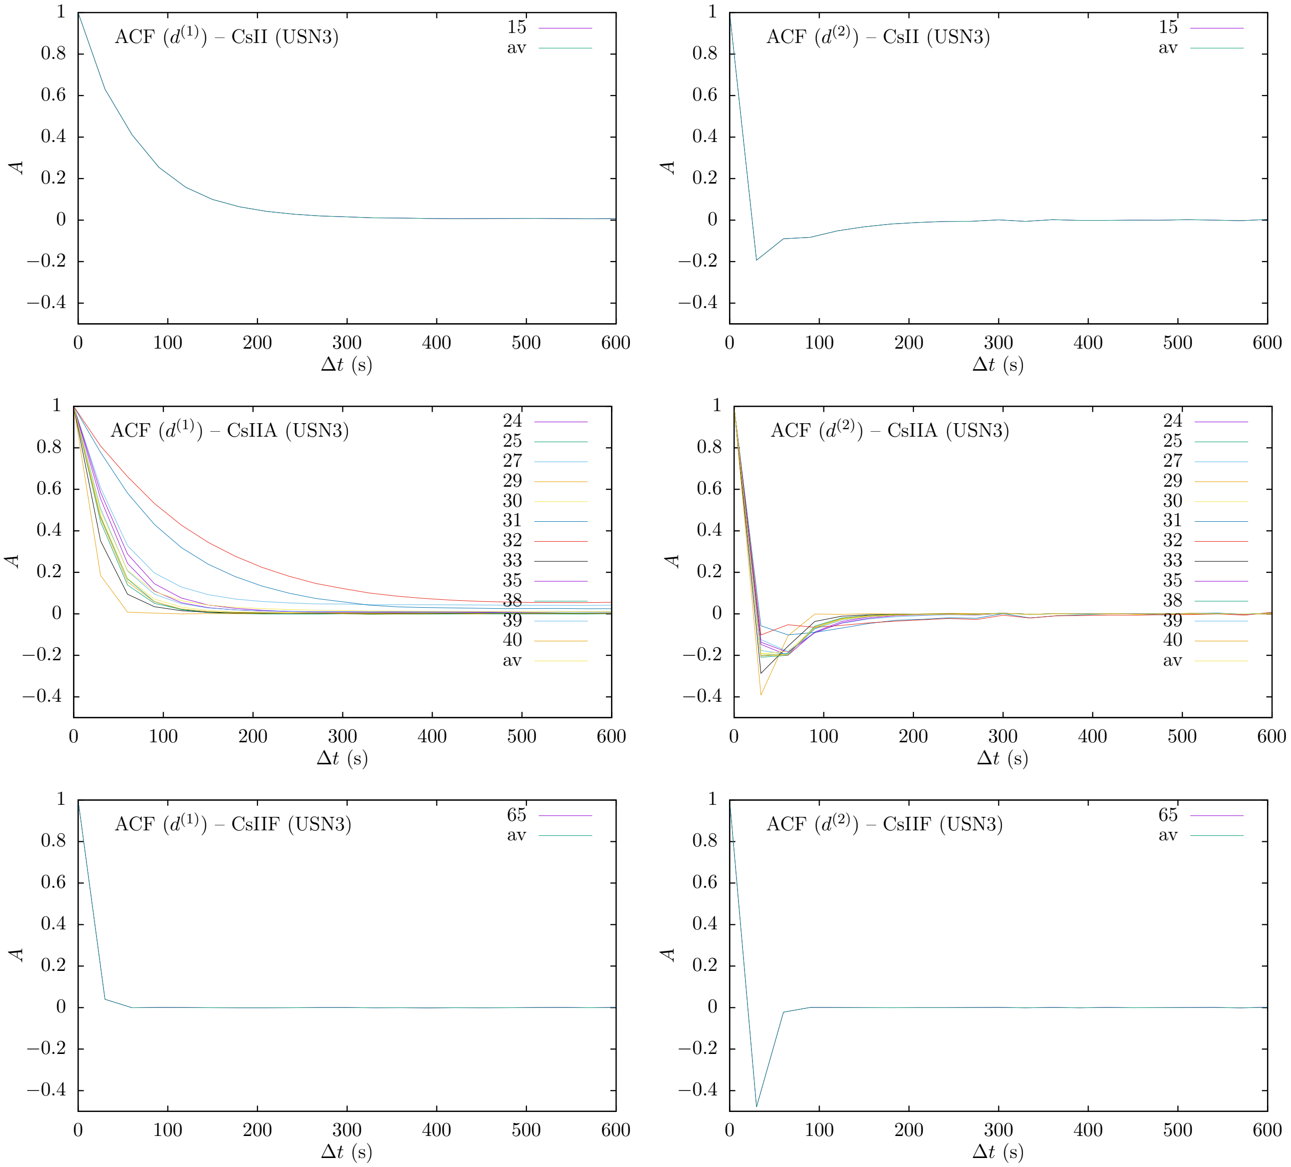


Figure 4: Cs autocorrelation functions, using (left) first- and (right) second-order differenced data. Each plot is for a particular Cs satellite block; each SVN is shown separately. Line labeled "av" is the average over all SNVs.

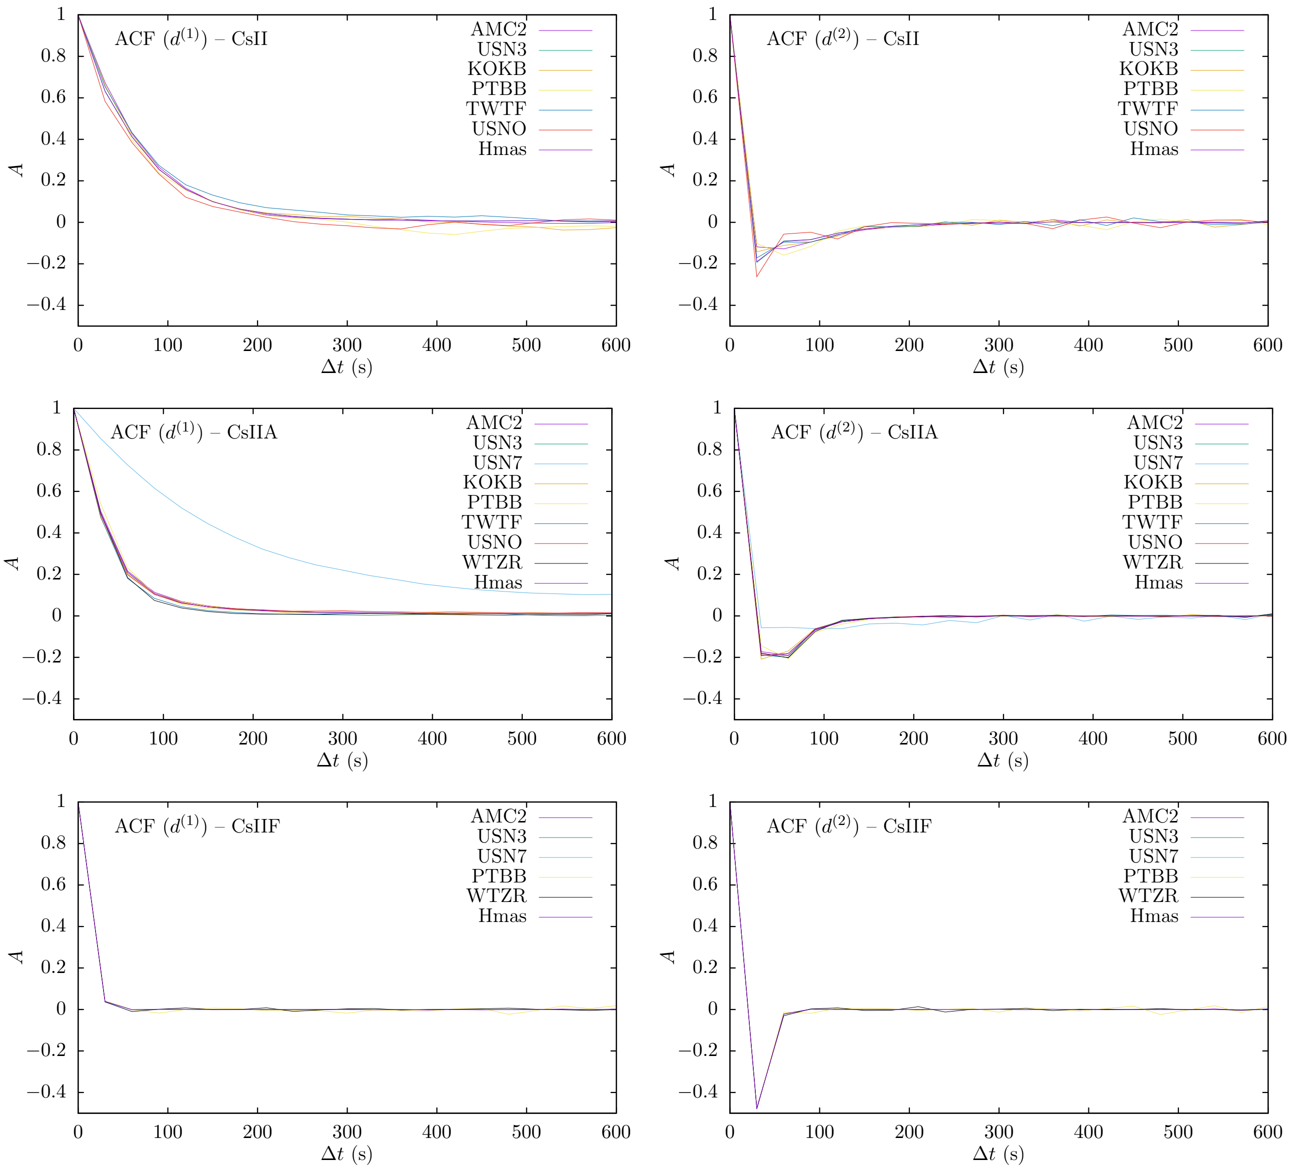


Figure 5: Cs autocorrelation functions, using (left) first- and (right) second-order differenced data. Each plot is for a particular Cs satellite block; each reference clock is shown separately. Line labeled "Hmas" is the average over all (H-maser) reference clocks.

# 3 Allan variance

$$\sigma_y^2(\Delta t) = \sum_{j=0}^{J-2\tau-1} \frac{\left(d_j - 2d_{j+\tau} + d_{j+2\tau}\right)^2}{2\tau^2\tau_0^2\,(J-2\tau)} \tag{4}$$

Here, $d_j = d_j^{(0)}$ – we use non-differenced data (after removal of 2nd order polynomial). For Rb, see Figs. 6–8. For Cs, see Figs. 9–10.

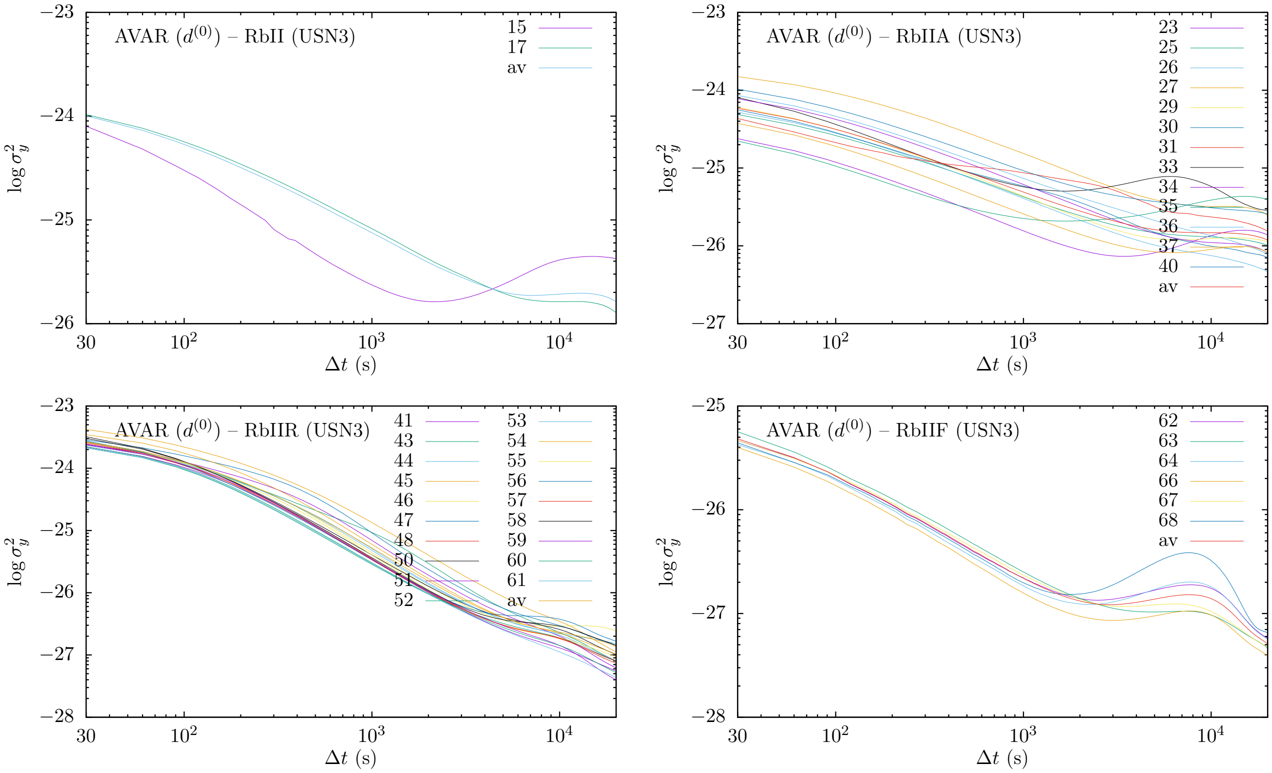


Figure 6: Rb Allan variance. Each plot is for a particular Rb satellite block; each SVN is shown separately. Line labelled "av" is the average over all SNVs.

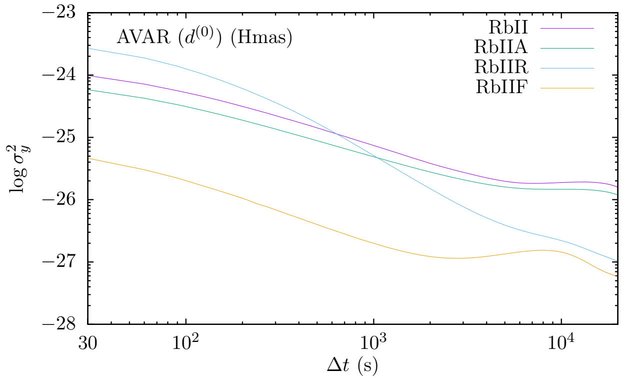


Figure 7: Rb Allan variance. Performance of each block averaged over each (H-maser) reference clocks.

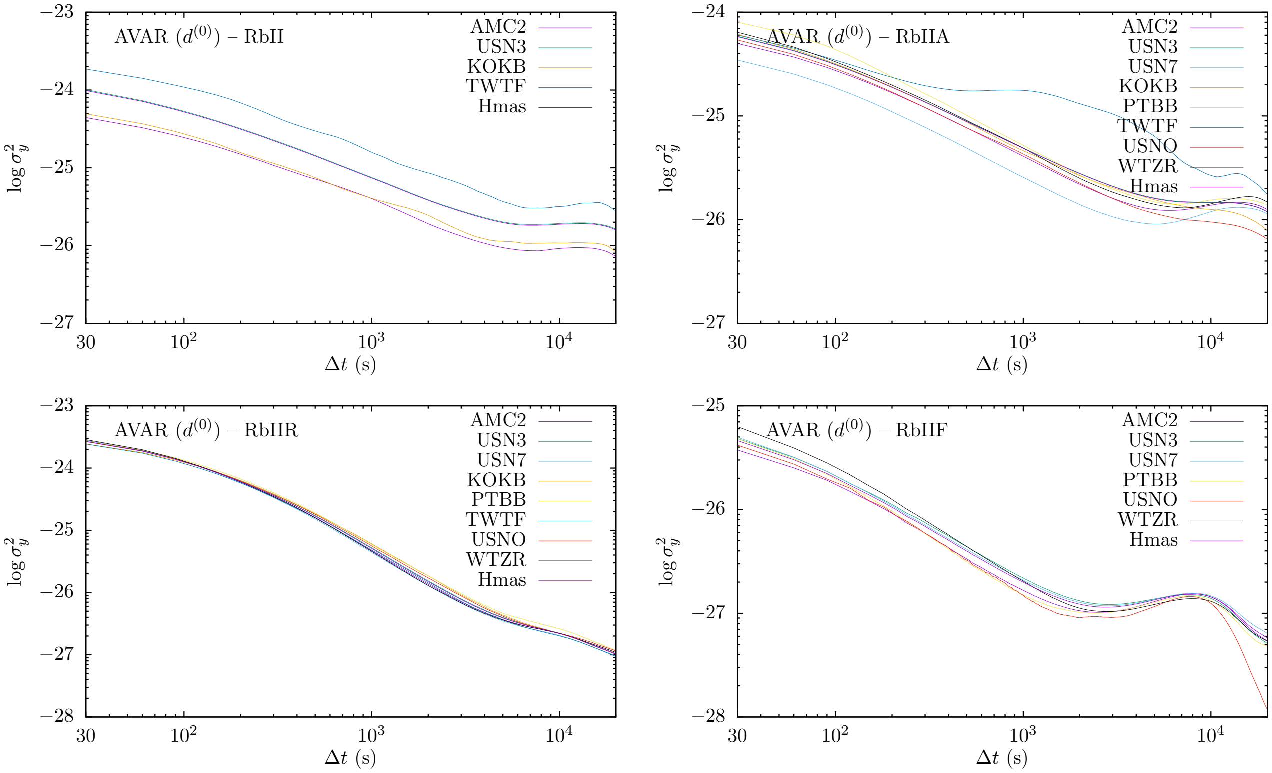


Figure 8: Rb Allan variance. Each plot is for a particular Rb satellite block; each reference clock is shown separately. Line labelled "Hmas" is the average over all (H-maser) reference clocks.

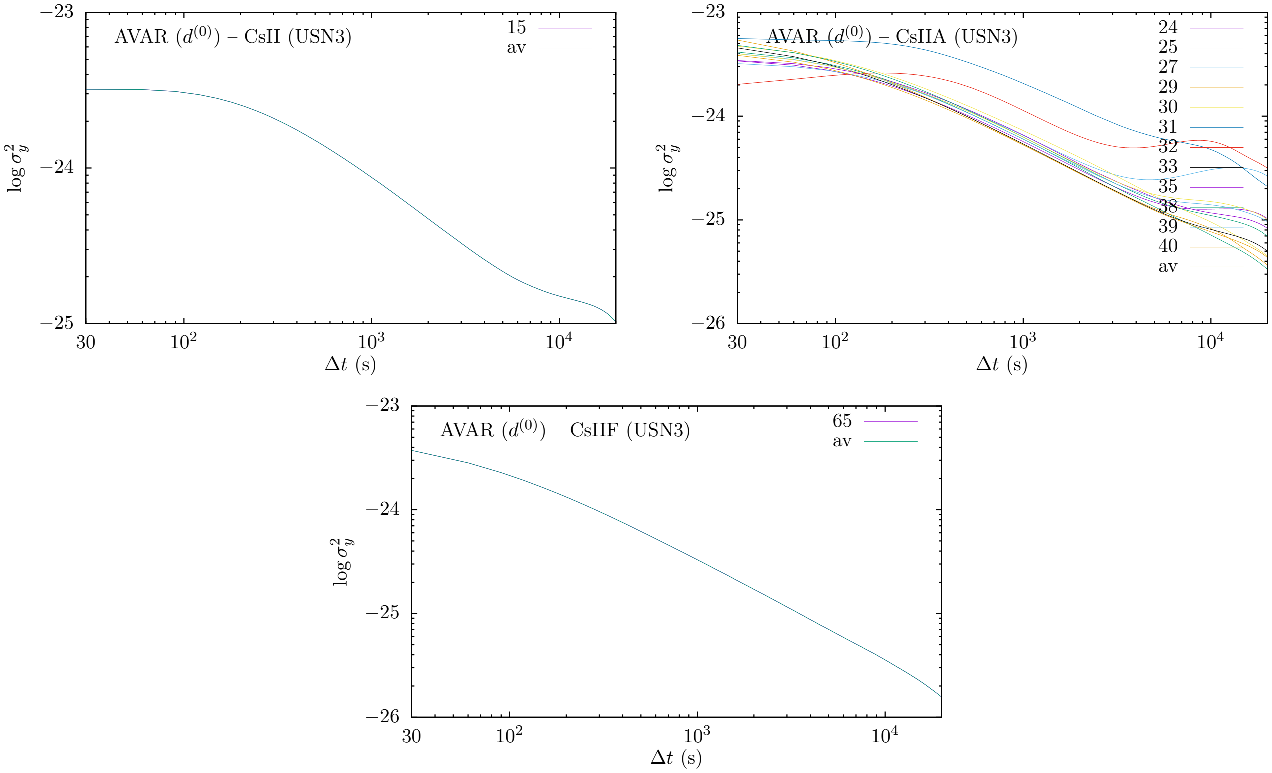


Figure 9: Cs Allan variance. Each plot is for a particular Cs satellite block; each SVN is shown separately. Line labelled "av" is the average over all SNVs.

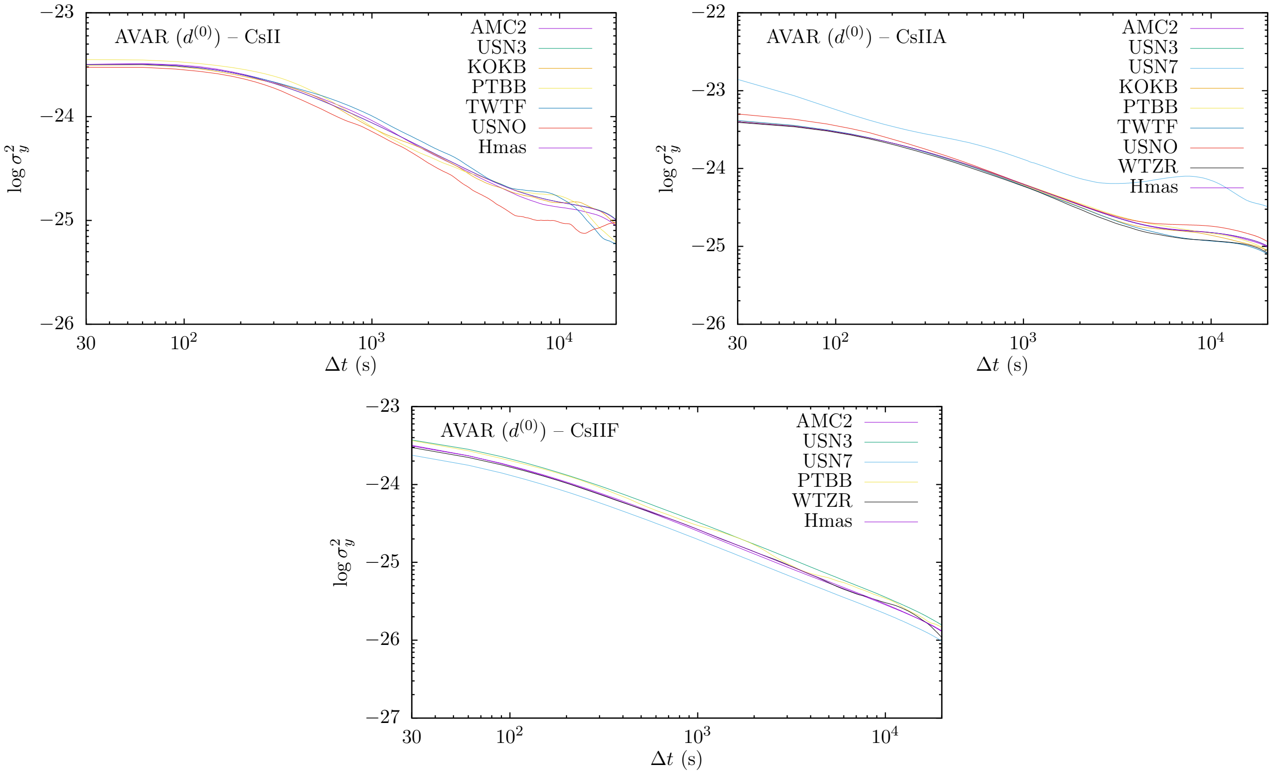


Figure 10: Cs Allan variance. Each plot is for a particular Cs satellite block; each reference clock is shown separately. Line labelled "Hmas" is the average over all (H-maser) reference clocks.

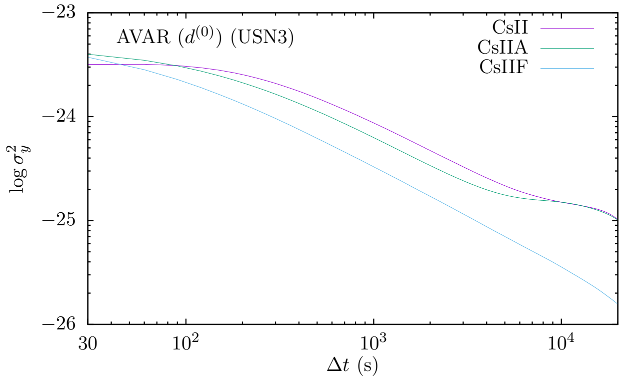


Figure 11: Cs Allan variance. Performance of each block for the USN3 reference.

# 4 Histogram

Count number of data points that fall into certain bins. Except where stated, uses the first-order differenced data, $d^{(1)}$. White noise should appear as a parabola on this log-scale. The bins range from $-1$ to $1\,\mathrm{ns}$, in equal steps of $0.001\,\mathrm{ns}$. Presented in units of counts per bin per epoch times bin-width.

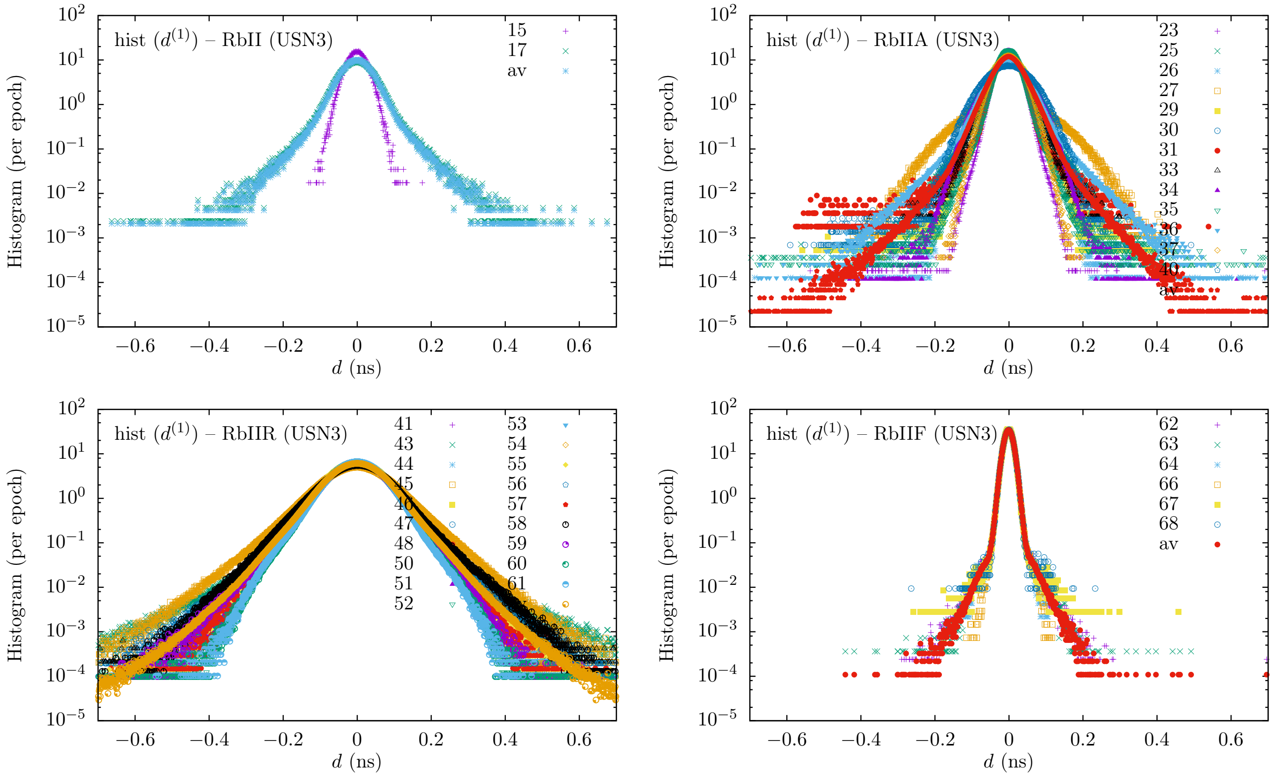


Figure 12: Rb histogram. Each plot is for a particular Rb satellite block; each SVN is shown separately. Line labeled "av" is the average over all SNVs.

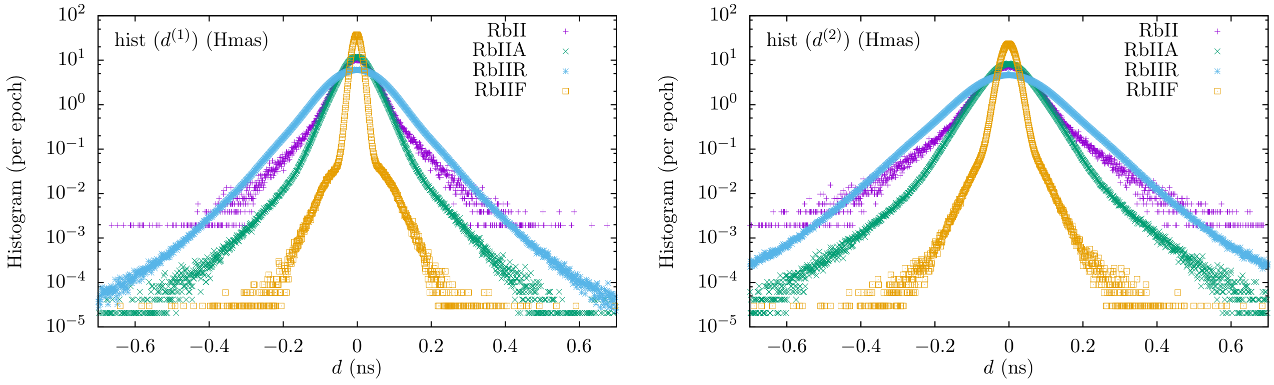


Figure 13: Rb histogram. Performance of each block averaged over each (H-maser) reference clocks. Left: first-order differenced data. Right: second-order differenced data.

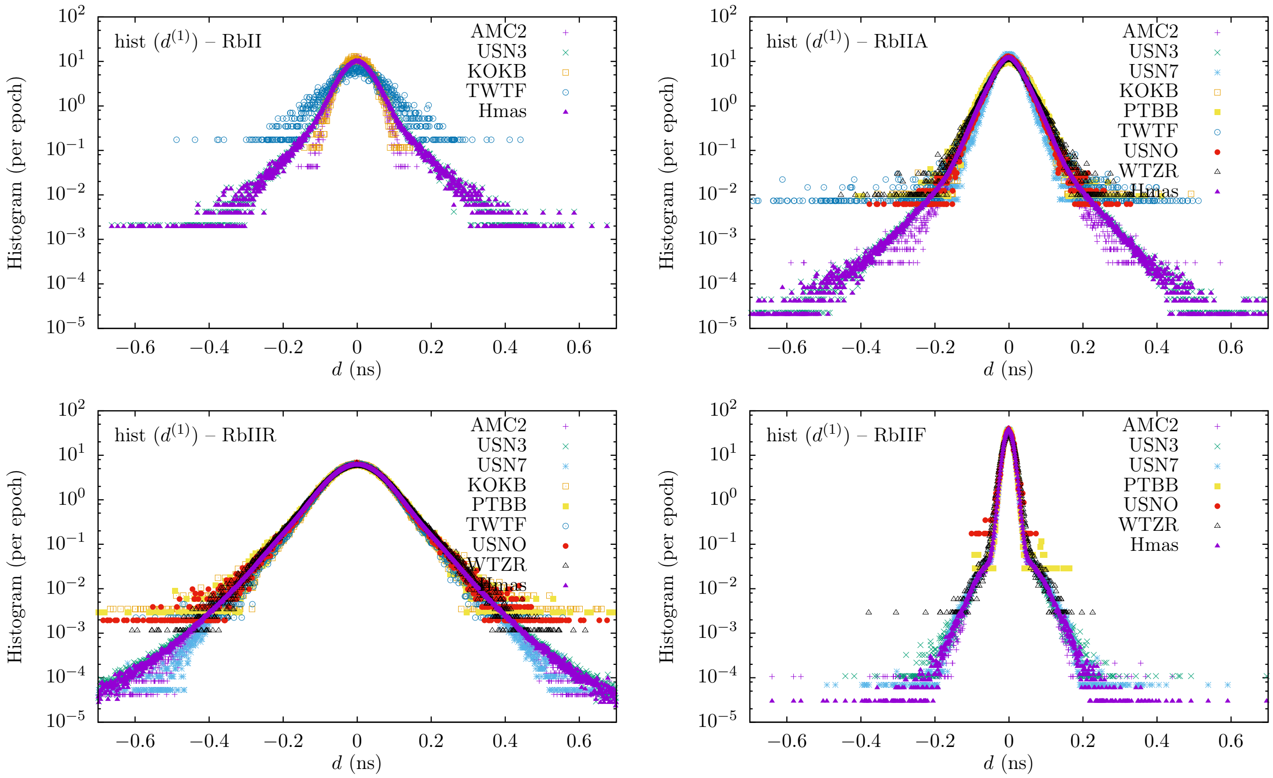


Figure 14: Rb histogram. Each plot is for a particular Rb satellite block; each reference clock is shown separately. Line labeled “Hmas” is the average over all (H-maser) reference clocks.

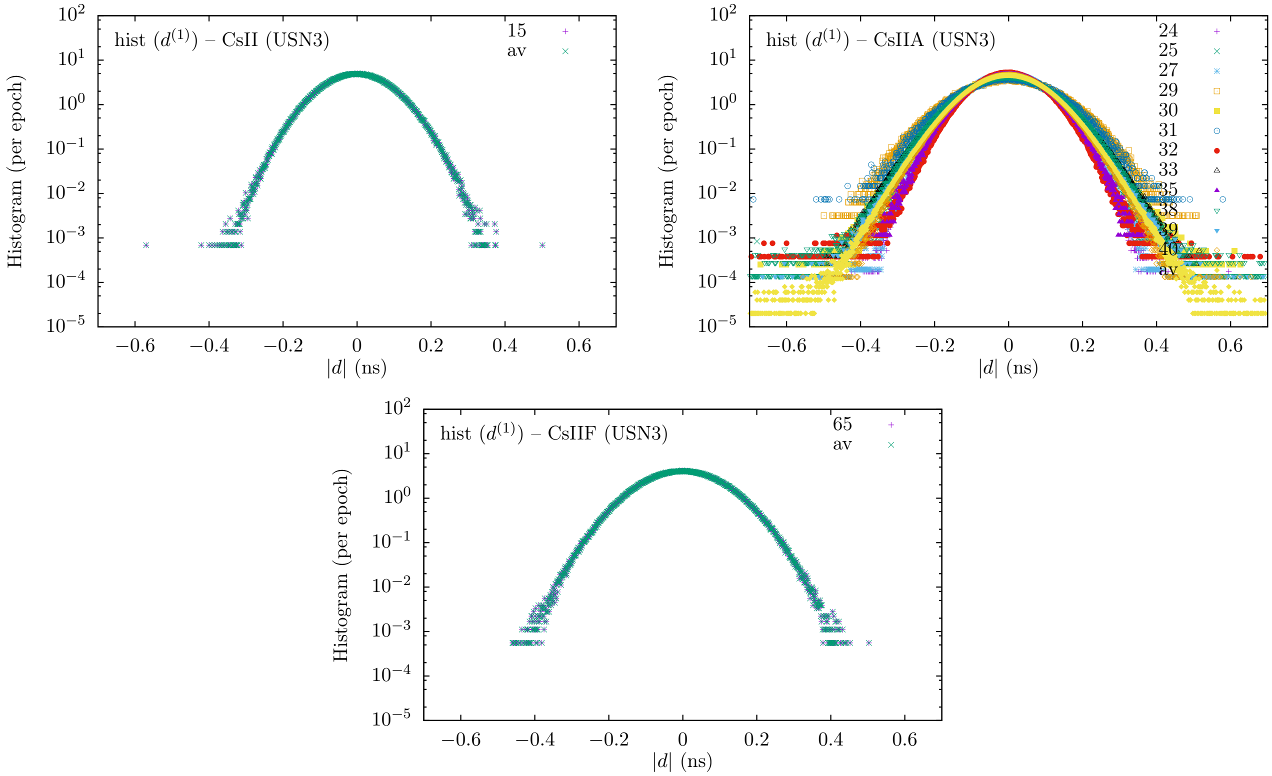


Figure 15: Cs histogram. Each plot is for a particular Cs satellite block; each SVN is shown separately. Line labeled “av” is the average over all SNVs.

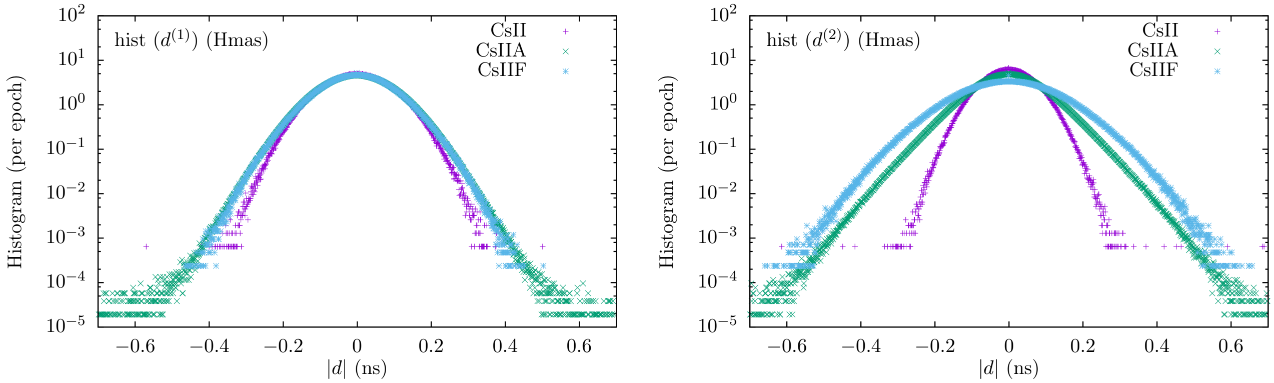


Figure 16: Cs histogram. Performance of each block averaged over each (H-maser) reference clocks. Left: first-order differenced data. Right: second-order differenced data.

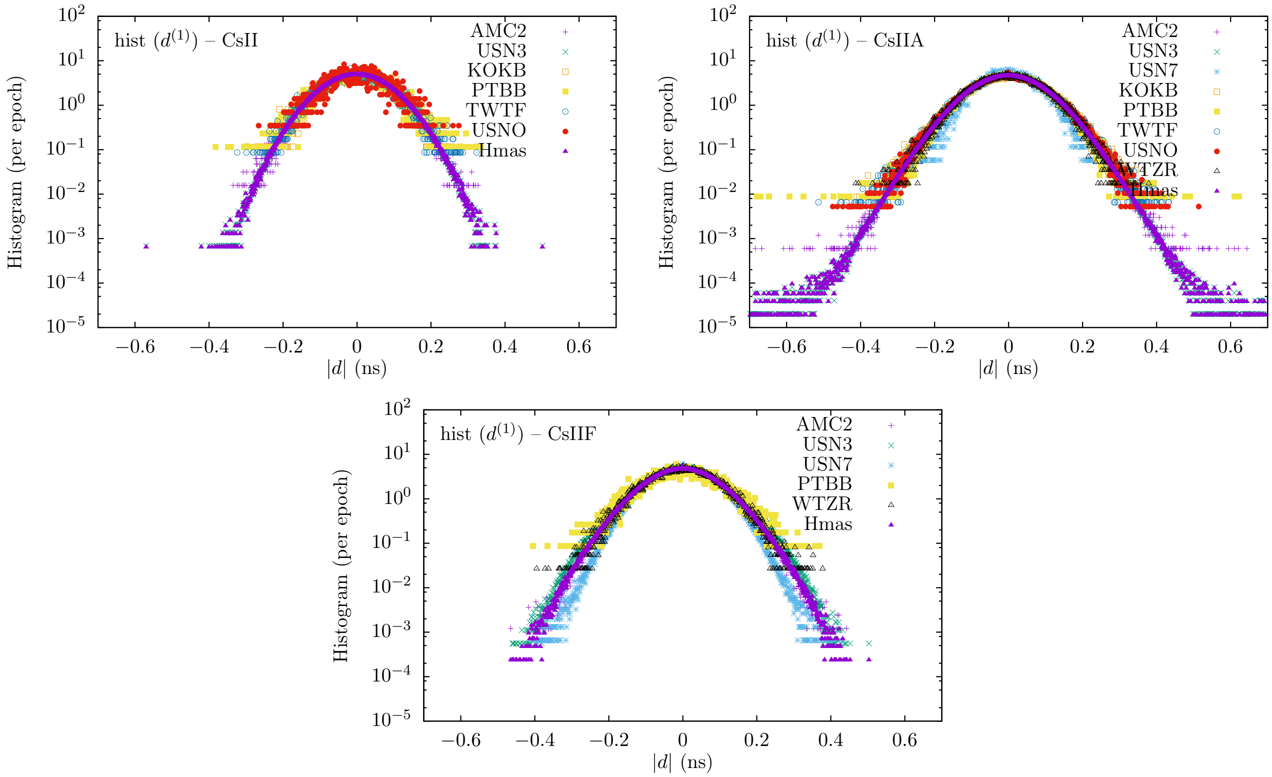


Figure 17: Cs histogram. Each plot is for a particular Cs satellite block; each reference clock is shown separately. Line labeled "Hmas" is the average over all (H-maser) reference clocks.

## 5 Power spectrums

For a given clock, $i$, we can form the power spectrum density (PSD),

$$S^i(k) = \frac{\tau_0}{J}\left|\widetilde{d^i}\right|^2, \tag{5}$$

where $\widetilde{d^i}$ is the discreet Fourier transform (DFT) of the clock time-series data for the $i$th clock.

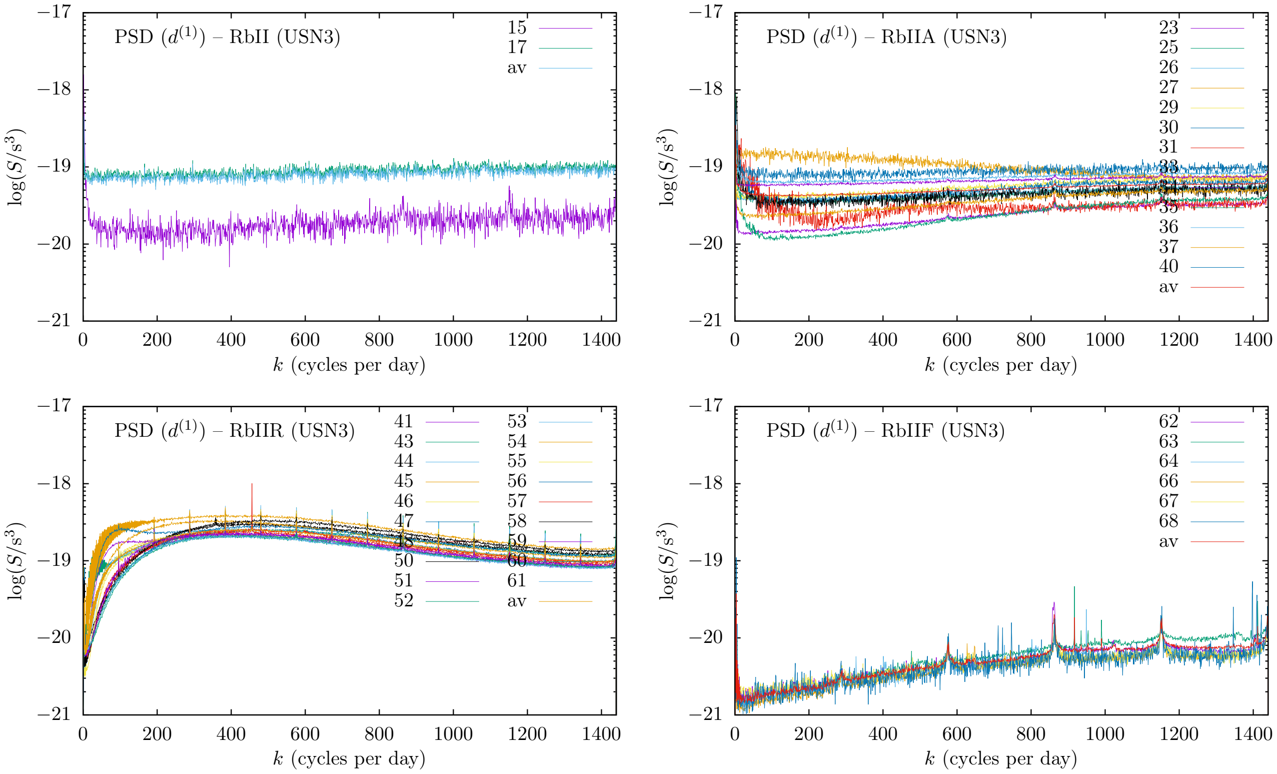


Figure 18: Rb power spectrums, using first-order differenced data. Each plot is for a particular Rb satellite block; each SVN is shown separately. Line labeled "av" is the average over all SNVs.

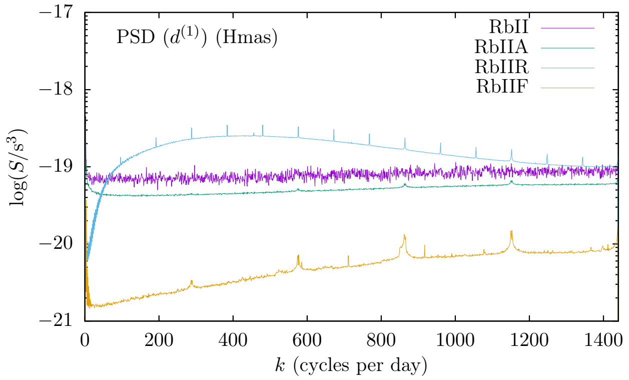


Figure 19: Rb power spectrums for each Rb satellite block, averaged over all SVN's and all (H-maser) reference clocks.

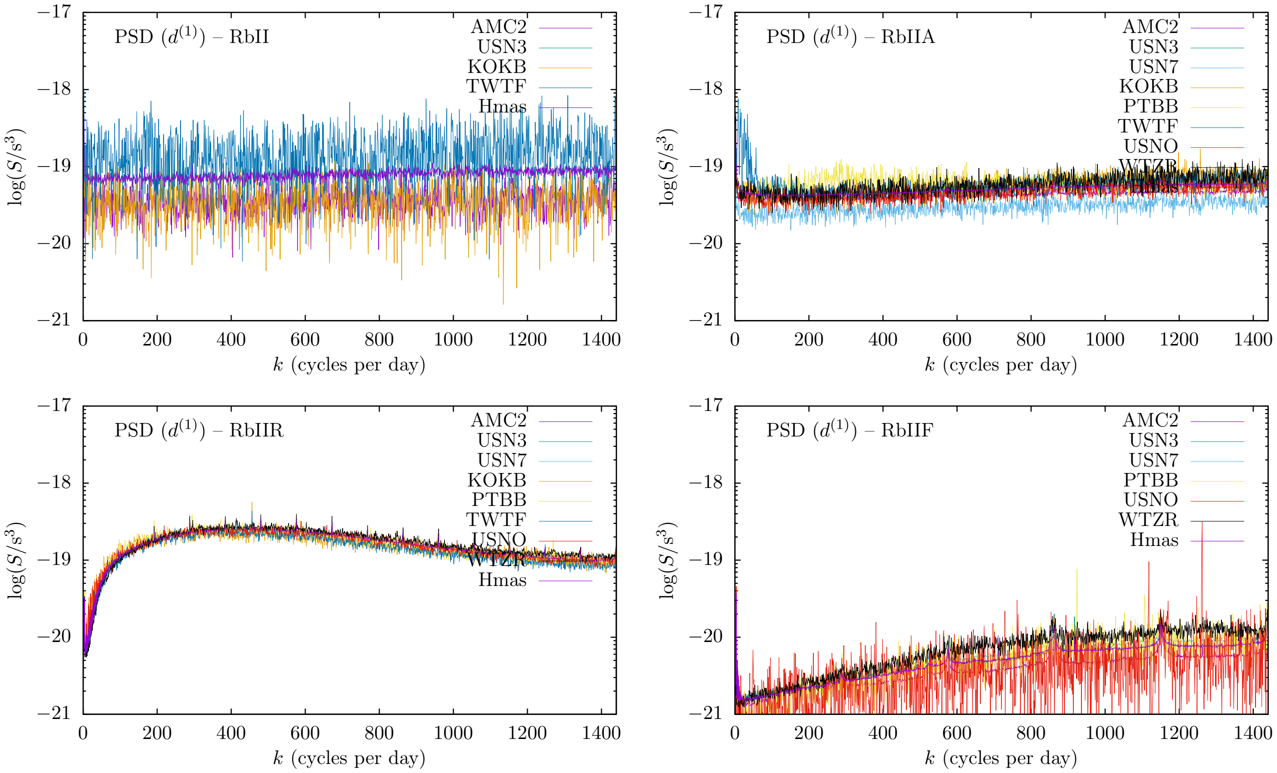


Figure 20: Rb power spectrums, using first-order differenced data. Each plot is for a particular Rb satellite block; each reference clock is shown separately. Line labeled "Hmas" is the average over all (H-maser) reference clocks.

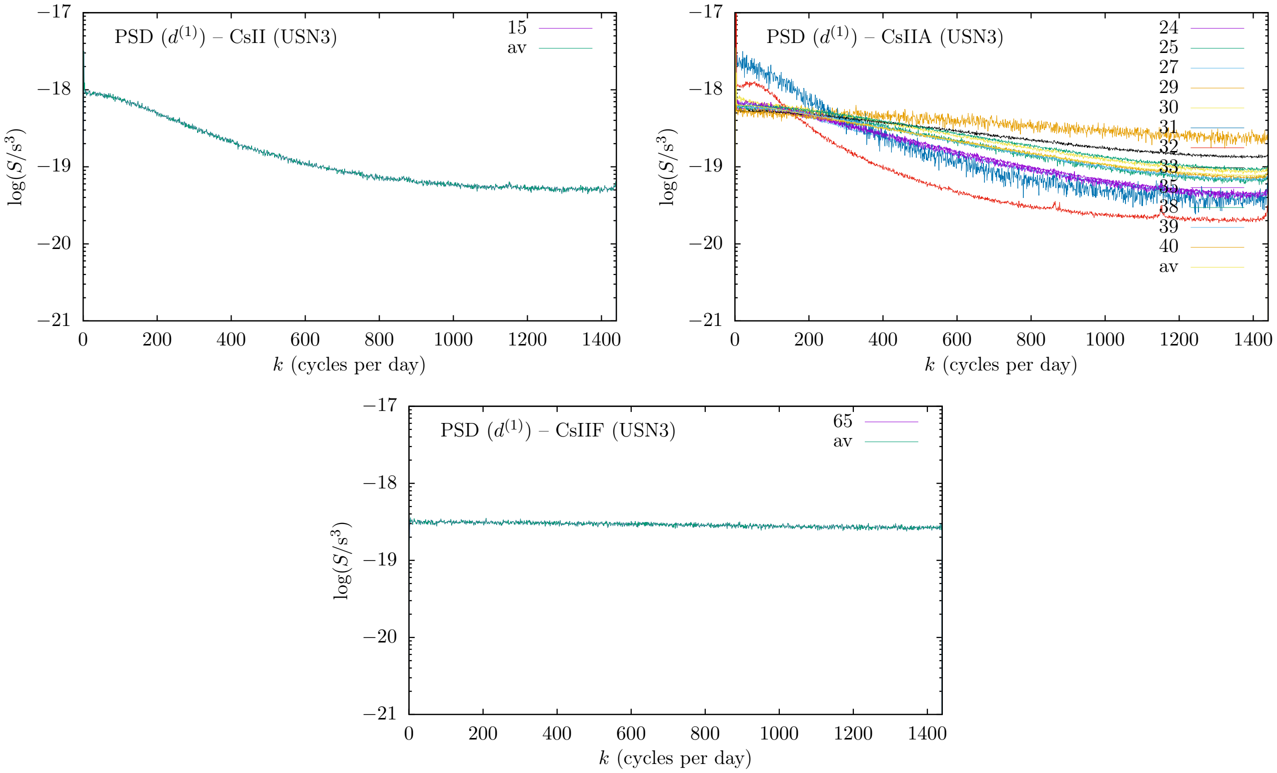


Figure 21: Cs power spectrums, using first-order differenced data. Each plot is for a particular Cs satellite block; each SVN is shown separately. Line labeled "av" is the average over all SNVs.

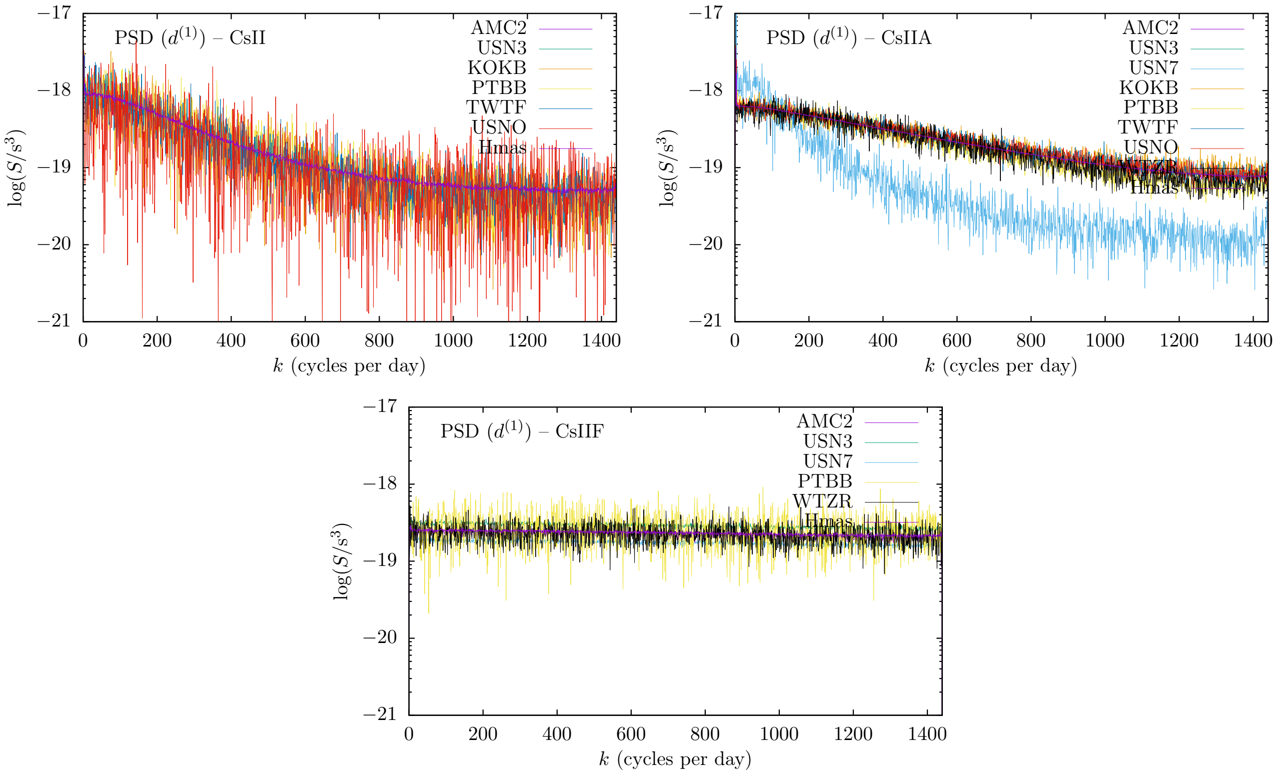


Figure 22: Cs power spectrums, using first-order differenced data. Each plot is for a particular Cs satellite block; each reference clock is shown separately. Line labeled “Hmas” is the average over all (H-maser) reference clocks.

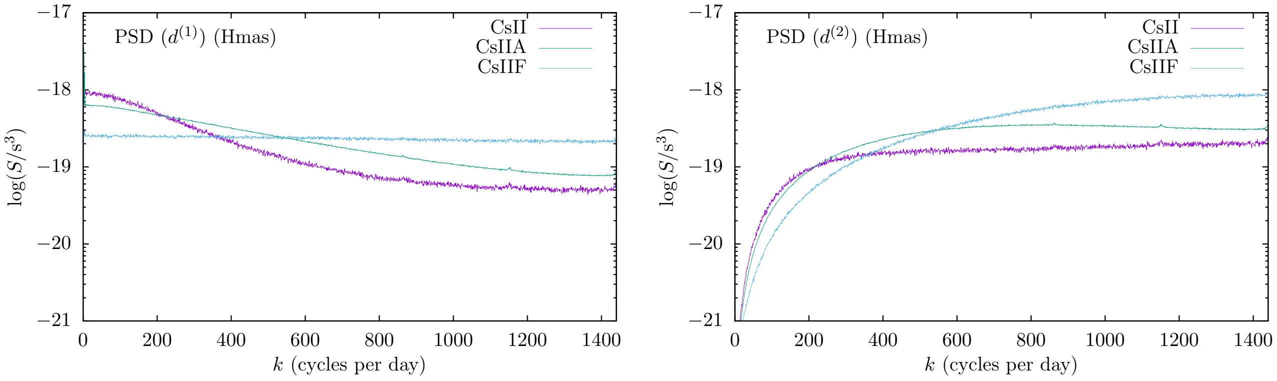


Figure 23: Cs power spectrums for each Cs satellite block, averaged over all SVN’s and all (H-maser) reference clocks, for first-order (left) and second-order (right) differenced data.

## 6 Cross-clock correlations

Here, the (zero-lag) cross-clock correlation is defined

$$C^{ik} \equiv \frac{\langle d_j^i d_j^k \rangle}{\sigma_i \sigma_k} = \frac{1}{J\,\sigma_i \sigma_k} \sum_j d_j^i d_j^k. \tag{6}$$

Presented are averages, defined:

$$C^i = \frac{1}{N} \sum_k C^{ik},$$

where (for brevity) the sum over $k$ runs only over clocks of the same type and block as clock $i$ (e.g., Rb-IIR). Calculations are for July 2004 – August 2017 (covering $144,203$ clock-days), and do not exclude any data. The results are shown in Tables 12 and 13 for the Rb and Cs clocks, respectively.

Table 12: Cross-clock correlations (at 0 lag) for Rb satellite clocks (averaged over all SVNs) for first- and second-order differenced data.

| Block | Ref. | Days | $C^{(1)}$ | $C^{(2)}$ |
|---|---|---|---|---|
| Rb IIA | AMC2 | 1497 | 0.026 | 0.030 |
| Rb IIA | USN3 | 19923 | 0.079 | 0.100 |
| Rb IIA | USN7 | 67 | 0.011 | 0.015 |
| Rb IIR | AMC2 | 10061 | 0.034 | 0.025 |
| Rb IIR | USN3 | 60801 | 0.035 | 0.036 |
| Rb IIR | USN7 | 10178 | 0.052 | 0.042 |
| Rb IIF | AMC2 | 3408 | 0.201 | 0.204 |
| Rb IIF | USN3 | 3459 | 0.267 | 0.274 |
| Rb IIF | USN7 | 5244 | 0.345 | 0.379 |

Table 13: Cross-clock correlations (at 0 lag) for Cs satellite clocks (averaged over all SVNs) for first- and second-order differenced data.

| Block | Ref. | Days | $C^{(1)}$ | $C^{(2)}$ |
|---|---|---|---|---|
| Cs IIA | AMC2 | 1151 | 0.003 | 0.010 |
| Cs IIA | USN3 | 22904 | 0.014 | 0.044 |
| Cs IIA | USN7 | 129 | 0.000 | 0.001 |
| Cs IIF | AMC2 | 626 | 0.002 | 0.002 |
| Cs IIF | USN7 | 1062 | 0.006 | 0.009 |

## References

[1] Jet Propulsion Laboratory, ftp://sideshow.jpl.nasa.gov/pub/jpligsac/

[2] PRN_GPS.gz, available at ftp://sideshow.jpl.nasa.gov/pub/gipsy_products/gipsy_params/

[3] US Navigation Center, https://www.navcen.uscg.gov/?Do=gpsArchives

[4] B. M. Roberts (2017), https://github.com/benroberts999/updatePRN_SVN
